# Supplementary material for: Hybrid Dealiased Convolutions
Source: arXiv:2306.10016 source file (2023-05-14)
Supplement: Supplementary file 1 [file appendix.tex]

\section{Appendix2}
%\addcontentsline{toc}{section}{Appendix}

\subsection{Python Code - 1D}

\begin{lstlisting}
#!/usr/bin/env python3

#Author: Robert Joseph George
# This file contains the 1D convolution code using the Hybrid Approach and compares it with the other
# state of the art FFT methods

from math import ceil
from cmath import exp,pi
import numpy as np
import scipy
from scipy import signal
import time
from functools import cache, reduce

def factors(n):
    return list(set(reduce(list.__add__,
                ([i, n//i] for i in range(1, int(n**0.5) + 1) if n % i == 0))))

def ceilquotient(a,b):
    return (a+b-1)//b

def mainconvolve(f,g,M,m,lambda1):
    L1,L2,N = len(f),len(g),len(g)
    Mf = m
    Mg = Mf*lambda1
    Pf = ceilquotient(L1,Mf)
    Pg = ceilquotient(L2,Mg)
    Qg = ceilquotient(M,Mg)
    Qf = lambda1*Qg
    Qm = Qf*Mf
    f = np.append(f,np.zeros(Pf*Mf-L1))
    g = np.append(g,np.zeros(Pg*Mg-L2))
    h_tilda = np.zeros(Pg*Mg, dtype = complex)
    for rg in range(Qg):
        g_tilda = np.zeros(Mg, dtype = complex)
        G_tilda = np.zeros(Mg, dtype = complex)
        for sg in range(Mg):
            sum1 = complex(0,0)
            for tg in range(min(Pg,ceilquotient((L2 - sg),Mg))):
                sum1 += g[tg*Mg + sg]*exp(2*pi*1j*tg*rg/Qg)
            g_tilda[sg] = sum1*exp(2*pi*1j*sg*rg/Qm)
        G_tilda = Mg*scipy.fft.ifft(g_tilda)
        F_tilda = np.zeros(Mg, dtype = complex)
        for lambda2 in range(lambda1):
            rf = lambda2*Qg + rg
            f_tilda = np.zeros(Mf, dtype = complex)
            for sf in range(Mf):
                sum1 = complex(0,0)
                for tf in range(min(Pf,ceilquotient((L1 - sf),Mf))):
                    sum1 += f[tf*Mf + sf]*exp(2*pi*1j*tf*rf/Qf)
                f_tilda[sf] = sum1*exp(2*pi*1j*sf*rf/Qm)
            f_tilda = Mf*scipy.fft.ifft(f_tilda)
            for lf in range(Mf):
                F_tilda[lambda1*lf + lambda2] = f_tilda[lf]
        H_tilda = np.zeros(Mg, dtype = complex)
        H_tilda = scipy.fft.fft(np.multiply(F_tilda,G_tilda))
        for s in range(Mg):
            H_tilda[s] = H_tilda[s]*np.conjugate(exp(2*pi*1j*s*rg/(Qg*Mg)))
        for t in range(Pg):
            for s in range(min(Mg,M - t*Mg)):
                h_tilda[t*Mg + s] += H_tilda[s]*np.conjugate(exp(2*pi*1j*t*rg/(Qg)))/(Qg*Mg)

    return h_tilda[0:N]

def forward(f, F, m, L, p, q, r, lambda1):
    Q = ceilquotient(M,m*lambda1)
    for lambda2 in range(lambda1):
        W = np.zeros(m, dtype = complex)
        R = Q*lambda2 + r
        for s in range(m):
            for t in range(p-1):
                W[s] += f[t*m + s]*exp((2*pi*1j*(t*m+s))*R/(q*m))
        for s in range(L - (p-1)*m):
            W[s] += f[(p-1)*m + s]*exp((2*pi*1j*(p-1)*m+s)*R/(q*m))
        f = scipy.fft(f)

def mainconvolve1(f,g,M,m,lambda1):
    L1,L2,N = len(f),len(g),len(g)
    Mf = m
    Mg = Mf*lambda1
    Pf = ceilquotient(L1,Mf)
    Pg = ceilquotient(L2,Mg)
    Qg = ceilquotient(M,Mg)
    Qf = lambda1*Qg
    Qm = Qf*Mf
    f = np.append(f,np.zeros(Pf*Mf-L1))
    g = np.append(g,np.zeros(Pg*Mg-L2))
    h_tilda = np.zeros(Pg*Mg, dtype = complex)
    for rg in range(Qg):
        g_tilda = np.zeros(Mg, dtype = complex)
        G_tilda = np.zeros(Mg, dtype = complex)
        for sg in range(Mg):
            sum1 = complex(0,0)
            for tg in range(min(Pg,ceilquotient((L2 - sg),Mg))):
                sum1 += g[tg*Mg + sg]*exp(2*pi*1j*tg*rg/Qg)
            g_tilda[sg] = sum1*exp(2*pi*1j*sg*rg/Qm)
        G_tilda = Mg*scipy.fft.ifft(g_tilda)
        F_tilda = np.zeros(Mg, dtype = complex)
        for lambda2 in range(lambda1):
            rf = lambda2*Qg + rg
            f_tilda = np.zeros(Mf, dtype = complex)
            for sf in range(Mf):
                sum1 = complex(0,0)
                for tf in range(min(Pf,ceilquotient((L1 - sf),Mf))):
                    sum1 += f[tf*Mf + sf]*exp(2*pi*1j*tf*rf/Qf)
                f_tilda[sf] = sum1*exp(2*pi*1j*sf*rf/Qm)
            f_tilda = Mf*scipy.fft.ifft(f_tilda)
            for lf in range(Mf):
                F_tilda[lambda1*lf + lambda2] = f_tilda[lf]
        H_tilda = np.zeros(Mg, dtype = complex)
        H_tilda = scipy.fft.fft(np.multiply(F_tilda,G_tilda))
        for s in range(Mg):
            H_tilda[s] = H_tilda[s]*np.conjugate(exp(2*pi*1j*s*rg/(Qg*Mg)))
        for t in range(Pg):
            for s in range(min(Mg,M - t*Mg)):
                h_tilda[t*Mg + s] += H_tilda[s]*np.conjugate(exp(2*pi*1j*t*rg/(Qg)))/(Qg*Mg)

    return h_tilda[0:N]

def direct(f,g):
    L1,L2 = len(f),len(g)
    H = np.zeros(L2,dtype = complex)
    for i in range(L2):
        sum1 = complex(0,0)
        for j in range(i+1):
            if i - j >= L2 or j >= L1:
                continue
            else:
                sum1 += f[j]*g[i-j]
        H[i] = sum1
    return H

def finalconvolve(f,g,M):
    f1 = factors(len(f))
    g1 = factors(len(g))
    best_m, best_lambda = 1,1
    best_time = 1e8
    for i in range(len(f1)):
        for j in range(len(g1)):
            start = time.time()
            mainconvolve(f,g,M,f1[i],g1[j])
            best = time.time() - start
            if(best < best_time):
                best_m = f1[i]
                best_lambda = g1[j]
                best_time = best
    print("Best time", best_time)
    return mainconvolve(f,g,M,best_m,best_lambda)

def randomfunction(m):
    f = []
    for i in range(m):
        f.append(complex(i,i+1))
    return f


N = 10
sum1, sum2, sum3 = 0,0,0
for i in range(N):
    f = np.array([1,2])
    g = np.array([1,2,3,4])

    start = time.time()
    direct(f,g)
    sum1 += time.time() - start

    start1 = time.time()
    signal.convolve(f,g,mode = "full")
    sum2 += time.time() - start1

    start2 = time.time()
    finalconvolve(f,g,len(f) + len(g) - 1)
    sum3 += time.time() - start2

print()
print(r"Direct Convolution {:g}".format((sum1)/N))
print(r"Convolution using Scipy FFT {:g}".format(sum2/N))
print(r"Convolution using Hybrid Approach {:g}".format(sum3/N))


\end{lstlisting}

\subsection{Python Code - 2D}

\begin{lstlisting}
    #!/usr/bin/env python3

# Author: Robert Joseph
# This file does an image convolution using the Hybrid approach.

from numpy.fft  import fft2, ifft2
import numpy as np
from pip import main
from scipy import signal
import scipy
from math import ceil
from cmath import exp,pi
from PIL import Image
import time
from functools import reduce
import os

mode_same_small = 1
mode_same_big = 2
mode_full = 3
mode_valid = 4

def np_fftconvolve(A, B):
    return ifft2(fft2(A)*fft2(B, s = A.shape))

def factors(n):
    return list(set(reduce(list.__add__,
                ([i, n//i] for i in range(1, int(n**0.5) + 1) if n % i == 0))))

def ceilquotient(a,b):
    return (a+b-1)//b

def forward(f,F,m,L,p,q,r,lambda1,M):
    Q = ceilquotient(M,lambda1*m)
    for lambda2 in range(lambda1):
        W = np.zeros(m,dtype=complex)
        R = Q*lambda2 + r
        for s in range(m):
            sum1 = complex(0,0)
            for t in range(p-1):
                sum1 += f[t*m + s]*exp(2*pi*1j*R*(t*m + s)/(q*m))
            W[s] = sum1
        for s in range(L - (p-1)*m):
            W[s] += f[(p-1)*m + s]*exp(2*pi*1j*R*((p-1)*m + s)/(q*m))
        W = m*scipy.fft.ifft(W)
        for l in range(m):
            F[lambda1*l + lambda2] = W[l]
    return F

def backward(F,f,m,L,p,q,r):
    W = scipy.fft.fft(F)
    for s in range(m):
        for t in range(q-1):
            f[t*m + s] += W[s] * np.conjugate(exp(2*pi*1j*(r*(t*m + s))/(q*m)))
    for s in range(L - (q-1)*m):
        f[(q-1)*m + s] += W[s]*np.conjugate(exp(2*pi*1j*(r*((q-1)*m + s))/(q*m)))
    return f

def mainconvolve(f,g,M,m,lambda1,choice = mode_same_big):
    L1 = len(f)
    L2 = len(g)
    N = L1 + L2 - 1
    Mf = m
    Mg = Mf*lambda1
    Pf = ceilquotient(L1,Mf)
    Pg = ceilquotient(L2,Mg)
    Qg = ceilquotient(M,Mg)
    Qf = lambda1*Qg
    Qm = Qf*Mf
    M1 = Qg*Mg
    m = Mg
    f = np.pad(array=f, pad_width=[0, Pf*Mf - L1], mode='constant', constant_values=0)
    g = np.pad(array=g, pad_width=[0, Pg*Mg - L2], mode='constant', constant_values=0)
    F = np.zeros(m,dtype=complex)
    G = np.zeros(m,dtype=complex)
    finalf = np.zeros((N,M1),dtype=complex)
    finalg = np.zeros((N,M1),dtype=complex)
    Hfinal1 = np.zeros((M1,M1),dtype=complex)
    Hfinal = np.zeros((M1,M1),dtype=complex)
    finalf1 = np.zeros((M1,M1),dtype=complex)
    finalg1 = np.zeros((M1,M1),dtype=complex)
    for i in range(L2):
        for r in range(Qg):
            if i < L1:
                finalf[i,r*m:(r+1)*m] = forward(f[i],F,Mf,L1,Pf,Qf,r,lambda1,M1)
            finalg[i,r*m:(r+1)*m] = forward(g[i],G,Mg,L2,Pg,Qg,r,1,M1)
    finalf = finalf.T
    finalg = finalg.T
    for i in range(M1):
        for r in range(Qg):
            finalf1[i][r*m:(r+1)*m] = forward(finalf[i],F,Mf,L1,Pf,Qf,r,lambda1,M1)
            finalg1[i][r*m:(r+1)*m] = forward(finalg[i],G,Mg,L2,Pg,Qg,r,1,M1)
    finalf1 = np.multiply(finalf1,finalg1)
    for i in range(M1):
        for r in range(Qg):
            Hfinal[i] = backward(finalf1[i][r*m:(r+1)*m],Hfinal[i],Mg,M1,Pg,Qg,r)
    Hfinal = Hfinal.T
    for i in range(M1):
        for r in range(Qg):
            Hfinal1[i] = backward(Hfinal[i][r*m:(r+1)*m],Hfinal1[i],Mg,M1,Pg,Qg,r)
    for i in range(M1):
        Hfinal1[i] = Hfinal1[i]/(Qm*Qm)
    v,v1 = 0,N
    if choice == mode_same_big:
        v1 = L2
    elif choice == mode_same_small:
        v,v1 = 1, 1+L1
    elif choice == mode_valid:
        v,v1 = ceil(N/L2) - 1, ceil(N/L1) + 1
    return Hfinal1[v:v1,v:v1]

def finalconvolve(f,g,M,choice = mode_same_big):
    f1 = factors(len(f))
    g1 = factors(len(g))
    f1.append(M)
    best_m, best_lambda = 1,1
    best_time = 1e8
    for i in range(len(f1)):
        for j in range(len(g1)):
            start = time.time()
            mainconvolve(f,g,M,f1[i],g1[j],choice)
            best = time.time() - start
            if(best < best_time):
                best_m = f1[i]
                best_lambda = g1[j]
                best_time = best
    print("Best time", best_time)
    return mainconvolve(f,g,M,best_m,best_lambda)

image = Image.open('Implicit-Image-convolve-2d'+os.sep+'Vd-Orig.png')

kernel = np.array([[0,0,0],[0,1,0],[0,0,0]],dtype=complex)
kernel1 = np.array([[-1,-1,-1],[-1,4,-1],[-1,-1,-1]],dtype=complex)
kernel2 = np.array([[-1,-1,-1],[-1,8,-1],[-1,-1,-1]],dtype=complex)
kernel3 = np.array([[0,-1,0],[-1,5,-1],[0,-1,0]],dtype=complex)
kernel4 = 1/9*(np.array([[1,1,1],[1,1,1],[1,1,1]],dtype=complex))
kernel5 = 1/16*(np.array([[1,2,1],[2,4,2],[1,2,1]],dtype=complex))
kernel6 = (1/256)*(np.array([[1,4,6,4,1],[4,16,24,16,4],[6,24,36,24,6],[4,16,24,16,4],[1,4,6,4,1]],dtype=complex))
kernel7 = (-1/256)*(np.array([[1,4,6,4,1],[4,16,24,16,4],[6,24,-476,24,6],[4,16,24,16,4],[1,4,6,4,1]],dtype=complex))

kernels_dict = {"Identity":kernel,"Ridge_detection_1":kernel1,"Ridge_detection_2":kernel2,"Sharpen":kernel3,"Box_blur":kernel4,"Gaussian_blur":kernel5,"Gaussian_blur_5":kernel6,"Unsharpen_masking":kernel7}

for k, v in kernels_dict.items():
    data = np.asarray(image,dtype=complex)
    image_result = np.zeros((data.shape),dtype=np.uint8)
    N = len(v) + len(data) - 1
    diff = N - 100
    for i in range(len(data[0][0])):
        image_result[:,:,i] = np.real(mainconvolve(v,data[:,:,i],128,len(v[0]),1,mode_full))[diff-1:N-1,1:N-1]
    Image.fromarray(image_result).save('Vd-Conv-' + k + "-final_convolve_optimized.png")

\end{lstlisting}
\subsection{Python Code - Optimization}

\begin{lstlisting}
    # %%

#!/usr/bin/env python3

import sys, getopt
import numpy as np
from math import *
import os
import subprocess
import shlex
import regex as re
import matplotlib.pyplot as plt
from mpl_toolkits.mplot3d import Axes3D
from collections import Counter

%matplotlib widget

def intersection_element(sets, threshold = 0.95):		
    c = Counter()
    for s in sets:
        for elem in s:
            c[elem] += 1
    return [k for k, v in c.items() if v >= len(sets) * threshold]

def sort_lists(A, B, k = 3):
	# Create a list of tuples where each tuple contains an element from A and its index in B
	zipped = list(zip(A, B, range(len(B))))

	# Sort the list of tuples based on the values in B
	zipped.sort(key=lambda x: x[1])

	# Create two separate lists from the sorted list of tuples
	sorted_A = [x[0] for x in zipped]
	sorted_B = [x[1] for x in zipped]
	indices = [x[2] for x in zipped]

	return sorted_A[:k], sorted_B[:k], indices[:k]

def sort_lists_eps(A, B, eps = 0.7):
	# Create a list of tuples where each tuple contains an element from A and its index in B
	zipped = list(zip(A, B, range(len(B))))

	# Sort the list of tuples based on the values in B
	zipped.sort(key=lambda x: x[1])

	t_best = zipped[0][1]
	t_worst = zipped[-1][1]

	threshold = t_best + eps*(t_worst - t_best)

	# Create two separate lists from the sorted list of tuples
	sorted_A = [x[0] for x in zipped if x[1] if x[1] <= threshold]
	sorted_B = [(x[1] - t_best)/(t_worst - t_best) for x in zipped if x[1]]

	return sorted_A, sorted_B

def match_pattern(pattern, line):
	m = []
	matches = re.findall(pattern, line)
	for match in matches:
		m.append(float(match[2:]))
	return m

def average_columns(data):
    # Transpose the 2D list to get the columns as rows
    transposed_data = [[row[i] for row in data] for i in range(len(data[0]))]

    # Calculate the sum of each column and divide by the number of rows
    result = [sum(column) / len(data) for column in transposed_data]

    return result

def intersection_confidence(final_m_values, final_time_values, k_values, threshold_values, k_method = True):
	for k in k_values:
		final_set = set()
		for c in range(len(final_m_values)):
			if k_method:
				final_m = sort_lists(final_m_values[c], final_time_values[c], k)
			else:
				final_m = sort_lists_eps(final_m_values[c], final_time_values[c], k)[0]
			if c == len(final_m_values) - 1:
				print("Final m values for square:", final_m)
			final_set.add(frozenset(final_m))

		for l in threshold_values:
			values = intersection_element(final_set, l)
			if len(values) != 0:
				if k_method:
					print("Common intersection of m values with threshold " + str(l) + " and k values " + str(k), values)
				else:
					print("Common intersection of m values with threshold " + str(l) + " and eps values " + str(k), values)
					
def optimal_values(final_m_values, final_time_values, point_to_compare = 0):
	final_set = []
	for c in range(len(final_m_values)):
		final_m = sort_lists(final_m_values[c], final_time_values[c], 1)[0]
		final_set.append(final_m - point_to_compare)
	return final_set

def shared_factors(num1, num2):
    # Find the smaller of the two numbers
    if num1 < num2:
        smaller = num1
    else:
        smaller = num2

    # Initialize a variable to keep track of the number of shared factors
    shared = 0

    # Check each number from 1 to the smaller number
    for i in range(1, smaller + 1):
        # If i is a factor of both num1 and num2, increment the shared variable
        if num1 % i == 0 and num2 % i == 0:
            shared += 1

    # Return the number of shared factors
    return shared


def plot2d(x,y,thread, threshold, point_to_compare):
	plt.title("Common intersection with threshold {} and point {}".format(threshold, point_to_compare))
	plt.xlabel("Ly values")
	plt.ylabel("Difference between the optimal value and the point to compare")
	plt.plot(x, y, label = "Thread " + str(thread))
	plt.savefig("threshold_" + str(threshold) + "_point_" + str(point_to_compare) + ".png")
	plt.show()

def plot(x,y,z,thread, plot_type = "3d"):
	# Create the figure and 3D axis
	fig = plt.figure(figsize = (10,10))
	if plot_type == "3d":
		ax = fig.add_subplot(111, projection='3d')
	else:
		ax = fig.add_subplot(111)

	# Plot the data
	colors = ['r', 'g', 'b', 'y', 'c', 'm', 'k', 'w'][:len(x)]

	optimal_t = []
	optimal_y = []
	for i in range(len(x)):
		max_time = float(1e5)
		max_m = 0
		for j in range(len(y[i])):
			if max_time > z[i][j]:
				max_m = y[i][j]
				max_time = z[i][j]
		optimal_t.append(max_time)
		optimal_y.append(max_m)
		
	print("Max upper bound on time:", max(optimal_t),"\n")
	print("Min upper bound on time:", min(optimal_t),"\n")
	print("Average upper bound on time:", sum(optimal_t)/len(optimal_t),"\n")

	print("Max m value:", max(optimal_y),"\n")
	print("Min m value:", min(optimal_y),"\n")
	print("Average m value:", sum(optimal_y)/len(optimal_y),"\n")

	if plot_type == "3d":
	
		for i in range(len(x)):
			ax.scatter(x[i], y[i], z[i], c=colors[i%8], marker='o')
			ax.text(x[i], optimal_y[i], optimal_t[i], "OP", size=10, zorder=1, color='k')
	
		#cb = plt.colorbar(ax1, pad=0.2)

		# Set axis labels
		ax.set_title('Time taken vs Ly and m values')
		#ax.set_xticks(x)
		ax.set_ylabel('m values')
		ax.set_zlabel('time taken values')
		ax.set_xlabel('Ly values')
	else:
		plt.scatter(x, optimal_y)
		plt.title('Optimal m values vs Ly values')
		plt.ylabel('m values')
		plt.xlabel('Ly values')
		#plt.yticks(optimal_y)

	# Show the plot
	#plt.savefig("test.png")
	plt.show()

# Function to generate multiples of the form 2^a * 3^b * 5^c * 7^d
def generate_multiples(a_max, b_max, c_max, d_max, bound):
    multiples = set()
    for a in range(a_max + 1):
        for b in range(b_max + 1):
            for c in range(c_max + 1):
                for d in range(d_max + 1):
                    multiple = 2**a * 3**b * 5**c * 7**d
                    if multiple <= bound:
                        multiples.add(multiple)
    return list(multiples)

# %%
lx_values = sorted(generate_multiples(a_max=10, b_max=10, c_max=10, d_max=10, bound = 2048))[1:]
print(lx_values)

# %% [markdown]
# # Main Results

# %%

thread = [[],[],[],[],[],[],[],[]]
lx_values = sorted(generate_multiples(a_max=10, b_max=10, c_max=10, d_max=10, bound = 2048))[49:50]
print(lx_values)
#lx_values = [j for j in range(2, 10)]
final_m_values = []
final_time_values = []
t_array = [1]
random_averages = 2

for l in lx_values:
	print("Lx=", l, end="\n")
	for thread in t_array:
		final_m_values = []
		final_time_values = []
		final_set = set()
		ly_values = sorted(generate_multiples(a_max=10, b_max=10, c_max=10, d_max=10, bound = l))[1:]
		for i in ly_values:
			print("Thread ", thread, ": ", end=" ")
			print("Ly=", i, end="\n")
			averaged_columns_m = []
			averaged_columns_time = []
			for k in range(random_averages):
				string = "./hybridconv2 -Lx=" + str(l) + " -Ly=" + str(i) + " -Mx=" + str(2*l) +" -My=" + str(2*i) + " -t -R -T=" + str(thread)
				print(string)
				cmd = subprocess.run(shlex.split(string), capture_output=True, text=True)
				string = cmd.stdout
				pattern = "m="
				matches = re.finditer(pattern, string)

				for match in matches:
					# Get the starting index of the match

					start = match.start()
					if int(start) < 100:
						# Get the line number by counting the number of newline characters before the match

						line_num = string[:start].count("\n") + 1
						line_start = string.rfind("\n", 0, start) + 1
						line_end = string.find("Optimal time: ", start)
						line = string[line_start:line_end]
 						# Extract the values as a float and append to a list
						m_values = match_pattern("m=\d+", line)
						time_values = match_pattern("t=[+-]?\d+(?:\.\d+)?(?:[eE][+-]?\d+)?", line)
						break
				
				averaged_columns_m.append(m_values[:7])
				averaged_columns_time.append(time_values[:7])
			final_m_values.append(average_columns(averaged_columns_m)[:7])
			final_time_values.append(average_columns(averaged_columns_time)[:7])
		print("-------------------------------------------------------")
		#plot(ly_values,final_m_values,final_time_values,thread)
		final_m_values = np.array(final_m_values)
		#print(final_m_values)
		final_time_values = np.array(final_time_values)
		#print(final_time_values)
		np.save("/home/rjoseph1/fftw++/tests/trial_runs/new_runs_final/final_square_m_values" + str(l), final_m_values)
		np.save("/home/rjoseph1/fftw++/tests/trial_runs/new_runs_final/final_square_time_values" + str(l), final_time_values)

# %%
final_m_values = np.load("final_m_values.npy")
final_time_values = np.load("final_time_values.npy")

# Best m values and how often they appear
z = optimal_values(final_m_values, final_time_values, 0)
r = Counter(z)

print("Optimal values for m:", r)

# Plot Ly_values vs m_values against the optimal 2d square
ly_values = [i for i in range(2,513)]
#plot(ly_values,final_m_values,final_time_values,thread,"2d")

plot(ly_values[400:], final_m_values[400:], final_time_values, thread=1, plot_type="2d")

# Final statistics
print("Final statistics:")

# final statistics for k = 3,5,7
#intersection_confidence(final_m_values, final_time_values, [3,5,7], [0.1,0.2,0.3,0.4,0.5,0.6,0.8,0.9], True)

# final statistcis for eps = 0.1,0.5,1
intersection_confidence(final_m_values, final_time_values, [0.1,0.2,0.5,0.6,0.9], [0.1,0.2,0.3,0.4,0.5,0.6,0.8,0.9], False)

# %%
e = "t=2.95e-07"
matches = re.findall("t=[+-]?\d+(?:\.\d+)?(?:[eE][+-]?\d+)?", e)
print(float(matches[0][2:]))

# %%
for i in [2,4,8,16,32,64,128,256]:
	print("Ly value = ", i)
	m, time = sort_lists_eps(final_m_values[i-1], final_time_values[i-1], 0.1)
	print("m values: ", m)
	print("time values: ", time)
	print("\n")

# %% [markdown]
# # Square optimal Values

# %%
final_square_m = np.load("final_square_m_values.npy")
final_square_time = np.load("final_square_time_values.npy")
final_square_m

# %%
def optimal_values(final_m_values, final_time_values, point_to_compare = 0):
	final_set = []
	for c in range(len(final_m_values)):
		final_m, time = sort_lists(final_m_values[c], final_time_values[c], 1)
		final_set.append(final_m - point_to_compare)
	return final_set

def final_comparison(point, bound = 2048, choice = False):
	square_size  = sorted(generate_multiples(a_max=10, b_max=10, c_max=10, d_max=10, bound = bound))[1:]
	index1 = square_size.index(point)
	if choice == True:
		range_index = input("Enter range choice")
		lower = int(range_index.split(" ")[0])
		upper = int(range_index.split(" ")[1])
	else:
		lower = index1 + 1
		upper = len(square_size)
	square_size  = sorted(generate_multiples(a_max=10, b_max=10, c_max=10, d_max=10, bound = bound))[lower:upper]
	final_best_m = []
	final_32_m = []
	final_best_time = []
	final_32_time = []
	final_32_indices = []
	final_best_indices = []
	for i in range(len(square_size)):
		print("Square size = ", square_size[i])
		final_square_m = np.load("/home/rjoseph1/fftw++/tests/trial_runs/new_final_runs/final_square_m_values" + str(square_size[i]) + ".npy").tolist()
		final_square_time = np.load("/home/rjoseph1/fftw++/tests/trial_runs/new_final_runs/final_square_time_values" + str(square_size[i]) + ".npy").tolist()
		sorted_m = []
		sorted_time = []
		ly_values = sorted(generate_multiples(a_max=10, b_max=10, c_max=10, d_max=10, bound = square_size[i]))[1:]
		index = ly_values.index(point)
		for j in range(len(final_square_m)):
			m, time, indices = sort_lists(final_square_m[j], final_square_time[j], 1)
			sorted_m.append(m)
			sorted_time.append(time)
		final_m, time, indices = sort_lists(sorted_m, sorted_time, 1)
		square, time2, indices1 = sort_lists(final_square_m[index], final_square_time[index], 1)
		final_best_m.append(final_m[0][0])
		final_32_m.append(square[0])
		final_best_time.append(time[0][0])
		final_32_time.append(time2[0])
		final_32_indices.append(32)
		final_best_indices.append(ly_values[indices[0]])
		print("{} Square best values".format(ly_values[indices[0]]), final_m[0], time[0])
		print("{} rectangle best values".format(square_size[index]), square, time2)
		print("----------------------------------------------------")

	# Create a figure with two subplots
	fig, (ax1, ax2, ax3) = plt.subplots(1, 3, figsize=(20, 10))

	# Plot m values on the left subplot
	ax1.plot(square_size, final_best_m, label='final_best_m')
	ax1.plot(square_size, final_32_m, label='final_{}_m'.format(point))
	ax1.set_xlabel('Lx value--->')
	ax1.set_ylabel('m value')
	ax1.legend()

	# Plot time values on the right subplot
	ax2.plot(square_size, final_best_time, label='final_best_time')
	ax2.plot(square_size, final_32_time, label='final_{}_time'.format(point))
	ax2.set_xlabel('Lx value--->')
	ax2.set_ylabel('time value')
	ax2.legend()

	# Plot time values on the right subplot
	ax3.plot(square_size, final_best_indices, label='final_best_Ly_values')
	ax3.plot(square_size, final_32_indices, label='final_{}_Ly_values'.format(point))
	ax3.set_xlabel('Lx value--->')
	ax3.set_ylabel('Best Rectangle size value')
	ax3.legend()
 
 	# Show the plot
	plt.show()
	plt.savefig("final_comparison_{}.png".format(point))

final_comparison(32, 2048, False)
#final_comparison(4, 2048)

# %%
def optimal_values(final_m_values, final_time_values, point_to_compare = 0):
	final_set = []
	for c in range(len(final_m_values)):
		final_m, time = sort_lists(final_m_values[c], final_time_values[c], 1)
		final_set.append(final_m - point_to_compare)
	return final_set

def final_comparison(point, bound = 2048, choice = False):
	square_size  = sorted(generate_multiples(a_max=10, b_max=10, c_max=10, d_max=10, bound = bound))[1:]
	index1 = square_size.index(point)
	if choice == True:
		range_index = input("Enter range choice")
		lower = int(range_index.split(" ")[0])
		upper = int(range_index.split(" ")[1])
	else:
		lower = index1 + 1
		upper = len(square_size)
	square_size  = sorted(generate_multiples(a_max=10, b_max=10, c_max=10, d_max=10, bound = bound))[index1+1:]
	final_best_m = []
	final_32_m = []
	final_best_time = []
	final_32_time = []
	final_32_indices = []
	final_best_indices = []
	square_final = []
	values = []
	square_best_m = []
	square_best_time = []
	for i in range(len(square_size)):
		#print("Square size = ", square_size[i])
		final_square_m = np.load("/home/rjoseph1/fftw++/tests/trial_runs/new_runs_final/final_square_m_values" + str(square_size[i]) + ".npy").tolist()
		final_square_time = np.load("/home/rjoseph1/fftw++/tests/trial_runs/new_runs_final/final_square_time_values" + str(square_size[i]) + ".npy").tolist()
		sorted_m = []
		sorted_time = []
		ly_values = sorted(generate_multiples(a_max=10, b_max=10, c_max=10, d_max=10, bound = square_size[i]))[1:]
		index = ly_values.index(point)
		#print(final_square_m[-1], final_square_time[-1])
		final_m, time, indices = sort_lists(final_square_m[-1], final_square_time[-1], 1)
		square, time2, indices1 = sort_lists(final_square_m[index], final_square_time[index], 1)
		if square[0] in final_square_m[-1]:
			square_final.append(square_size[i])
			#print("Square value is in the final m values", square[0])
			index = final_square_m[-1].index(square[0])
			time1 = final_square_time[-1][index]
			square1 = final_square_m[-1][index]
			indices = square_size[i]

			final_best_m.append(square1)
			final_32_m.append(final_m[0] )
			final_best_time.append(time1)
			final_32_time.append(time2[0])
   
			final_m, time, indices = sort_lists(final_square_m[-1], final_square_time[-1], 1)
			square_best_m.append(final_m[0])
			square_best_time.append(time[0])

			#print("{} Square best values".format(indices), final_m[0], time)
			#print("{} Square ml  values".format(square_size[0]), square1 , time1 )
			#print("----------------------------------------------------")
			 

	square_size = square_final
	# Create a figure with two subplots
	fig, (ax1, ax2) = plt.subplots(1, 2, figsize=(15, 10))
 
	# Plot m values on the left subplot
	#ax1.scatter(square_size, final_32_m, label='rectangle_ml_32')
	ax1.scatter(square_size, final_best_m, label='square_{}_m'.format(point), marker='x')
	ax1.scatter(square_size, square_best_m, label='square_best_m', marker = '+')
	ax1.set_xlabel('Lx value--->')
	ax1.set_ylabel('m value')
	ax1.legend()

	# Plot time values on the right subplot
	#ax2.scatter(square_size, final_32_time, label='rectangle_time_ML32')
	ax2.scatter(square_size, final_best_time, label='square_{}_time'.format(point), marker='x' )
	ax2.scatter(square_size, square_best_time, label='square_best_time', marker = '+')
	ax2.set_xlabel('Lx value--->')
	ax2.set_ylabel('time (seconds) - Log scale')
	ax2.set_yscale('log')
	ax2.legend()

 	# Show the plot
	plt.show()
	plt.savefig("final_comparison_{}.png".format(point))

final_comparison(32, 2048, False)

# %%
square_size = sorted(generate_multiples(a_max=10, b_max=10, c_max=10, d_max=10, bound = 2048))[10:]
for i in range(len(square_size)): 	
   final_square_m = np.load("/home/rjoseph1/fftw++/tests/trial_runs/new_runs_final/final_square_m_values" + str(square_size[i]) + ".npy").tolist()
   final_square_time = np.load("/home/rjoseph1/fftw++/tests/trial_runs/new_runs_final/final_square_time_values" + str(square_size[i]) + ".npy").tolist()
   print(square_size[i], final_square_m[-1], final_square_time[-1])

# %%
def square_optimal(square_size, threshold, epsilon):
    array3 = []
    for a in range(len(epsilon)):
        print("Epsilon = ", epsilon[a])
        print("******************************************************", end="\n")
        array2 = []
        for i in range(len(square_size)):
            print("Square size = ", square_size[i])
            final_square_m = np.load("final_square_m_values" + str(square_size[i]) + ".npy").tolist()
            final_square_time = np.load("final_square_time_values" + str(square_size[i]) + ".npy").tolist()
            final_best_square_m = np.load("final_square_m_values.npy")
            final_best_square_time = np.load("final_square_time_values.npy")
            best_m = sort_lists(final_best_square_m[i], final_best_square_time[i], 1)[0]
            array1 = []
            for j in range(2,square_size[i]):
                if shared_factors(j, square_size[i]) > threshold:
                    m = sort_lists_eps(final_square_m[j-1], final_square_time[j-1], epsilon[a])[0]
                    if best_m in m:
                        print("Ly value = ", j)
                        array1.append(j)
            if len(array1) == 0:
                print("No Ly values found.")
                array1.append(0)
            array2.append(array1)
            print("------------------------------------------------------")
        array3.append(array2)
    return array3

epsilon = [0.05]
square_size = [16,32,64,128,256,512,1024]
threshold = 2
array3 = square_optimal(non_optimal_square_size, threshold, epsilon)

# %%
def square_optimal(square_size, threshold, epsilon, choice = 0):
    array3 = []
    for a in range(len(epsilon)):
        print("Epsilon = ", epsilon[a])
        print("******************************************************", end="\n")
        array2 = []
        array_final = []
        array_x = []
        for i in range(len(square_size)):
            print("Square size = ", square_size[i])
            if choice == 0:
                final_square_m = np.load("/home/rjoseph1/fftw++/tests/trial_runs/new_final_runs/final_square_m_values" + str(square_size[i]) + ".npy").tolist()
                final_square_time = np.load("/home/rjoseph1/fftw++/tests/trial_runs/new_final_runs/final_square_time_values" + str(square_size[i]) + ".npy").tolist()
            elif choice == 1:
                final_square_m = np.load("/home/rjoseph1/fftw++/tests/trial_runs/final_runs1/final_square_m_values" + str(square_size[i]) + ".npy").tolist()
                final_square_time = np.load("/home/rjoseph1/fftw++/tests/trial_runs/final_runs1/final_square_time_values" + str(square_size[i]) + ".npy").tolist()
            elif choice == 2:
                final_square_m = np.load("/home/rjoseph1/fftw++/tests/trial_runs/final_runs2/final_square_m_values" + str(square_size[i]) + ".npy").tolist()
                final_square_time = np.load("/home/rjoseph1/fftw++/tests/trial_runs/final_runs2/final_square_time_values" + str(square_size[i]) + ".npy").tolist()      
            best_m = sort_lists(final_square_m[-1], final_square_time[-1], 1)[0]
            array1 = []
            values_to = sorted(generate_multiples(a_max=10, b_max=10, c_max=10, d_max=10, bound = square_size[i]))[1:]
            c = 0
            for j in values_to:
                if shared_factors(j, square_size[i]) > threshold:
                    m, n = sort_lists_eps(final_square_m[c], final_square_time[c], epsilon[a])
                    if best_m[0] in m:
                        print("Ly value = ", j)
                        array1.append(j)
                        array_final.append(array1)
                        array_x.append(square_size[i])
                c += 1
            if len(array1) == 0:
                print("No Ly values found.")
                array1.append(0)
            array2.append(array1[:1])
            print("------------------------------------------------------")
        array3.append(array2)
    return array3, array_final, array_x

# Example usage
epsilon = [0.01]
non_optimal_square_size =  sorted(generate_multiples(a_max=10, b_max=10, c_max=10, d_max=10, bound = 2048))[2:] #list(filter(lambda x: x in multiples, values))
threshold = 2
array3, array_final, array_x = square_optimal(non_optimal_square_size, threshold, epsilon, choice = 0)

# %%
c,d = 0,0
for i in range(len(array_final)):
	if array_x[i] % array_final[i][0] == 0:
		print(array_x[i], array_final[i], "divisible")
		c += 1
	else:
		print(array_x[i], array_final[i], "not divisible")
		d +=1 
print(c, d)

# %%
# old code
y = array3
x = non_optimal_square_size

fig, axs = plt.subplots(2, 4, figsize=(19, 9.2), gridspec_kw={'wspace': 0.5, 'hspace': 0.5})
r = 0
for j in range(len(epsilon)):
    if j == 4:
        r = 1
    for i in range(len(non_optimal_square_size)):
        if y[j][i] == [0]:
            axs[r][j%4].scatter([x[i]]*len(y[j][i]), y[j][i], color = 'blue')
        else:
            axs[r][j%4].scatter([x[i]]*len(y[j][i]), y[j][i], label = "Epsilon = " + str(epsilon[j]), color = 'red')

    axs[r][j%4].set_xlabel('Square size --->')
    axs[r][j%4].set_ylabel('Smallest rectangle Ly value --->')
    axs[r][j%4].set_title('Epislon = ' + str(epsilon[j]) + ' and threshold = ' + str(threshold))

plt.show()

# %%
import matplotlib.cm as cm
from matplotlib.cm import ScalarMappable
import matplotlib.patches as mpatches

y = array3
x = non_optimal_square_size

fig, axs = plt.subplots(2, 4, figsize=(19, 9.2), gridspec_kw={'wspace': 0.3, 'hspace': 0.3})
for j in range(len(epsilon)):
    color_dict = {}
    for i in range(len(non_optimal_square_size)):
        y_value = y[j][i][0]
        if y_value in color_dict:
            color_dict[y_value].append((x[i], y_value))
        else:
            color_dict[y_value] = [(x[i], y_value)]
    count_dict = {}
    for y_value in color_dict.keys():
        count = len(color_dict[y_value])
        if count in count_dict:
            count_dict[count].append(y_value)
        else:
            count_dict[count] = [y_value]
    sorted_counts = sorted(count_dict.keys(), reverse=True)
    group_dict = {}
    color_idx = 0
    for count in sorted_counts:
        y_values = count_dict[count]
        if len(y_values) == 1:
            group_dict[y_values[0]] = cm.Blues(color_idx/len(count_dict))
            color_idx += 1
        else:
            group_color = cm.Blues(color_idx/len(count_dict))
            for y_value in y_values:
                group_dict[y_value] = group_color
            color_idx += 1
    handles = []
    for y_value in sorted(color_dict.keys(), key=lambda x: len(color_dict[x]), reverse=True):
        handles.append(mpatches.Patch(color=group_dict[y_value], label=f'{y_value} ({len(color_dict[y_value])})'))
        for point in color_dict[y_value]:
            axs[j//4][j%4].scatter([point[0]], point[1], color=group_dict[y_value])
    axs[j//4][j%4].set_xlabel('Square size --->')
    axs[j//4][j%4].set_ylabel('Ly value --->')
    axs[j//4][j%4].set_title('Epsilon = ' + str(epsilon[j]))
    sm = ScalarMappable(cmap=cm.Blues, norm=plt.Normalize(vmin=0, vmax=len(count_dict)))
    sm.set_array([])
    #plt.colorbar(sm, orientation='vertical')
axs[j//4][j%4].legend(title = "Frequency sort by colors", handles=handles, loc = 'upper left', bbox_to_anchor=(1, 1.8))

plt.show()


# %%
# plot by plot
import matplotlib.cm as cm
from matplotlib.cm import ScalarMappable
import matplotlib.patches as mpatches

y = array3
x = non_optimal_square_size
plt.figure(figsize=(13, 10))
r = 0
color_dict = {}
for j in range(len(epsilon)):
    for i in range(len(non_optimal_square_size)):
        y_value = y[j][i][0]
        if y_value in color_dict:
            color_dict[y_value].append((x[i], y_value))
        else:
            color_dict[y_value] = [(x[i], y_value)]
    count_dict = {}
    for y_value in color_dict.keys():
        count = len(color_dict[y_value])
        if count in count_dict:
            count_dict[count].append(y_value)
        else:
            count_dict[count] = [y_value]
    sorted_counts = sorted(count_dict.keys(), reverse=True)
    group_dict = {}
    color_idx = 0
    for count in sorted_counts:
        y_values = count_dict[count]
        if len(y_values) == 1:
            group_dict[y_values[0]] = cm.Blues(color_idx/len(count_dict))
            color_idx += 1
        else:
            group_color = cm.Blues(color_idx/len(count_dict))
            for y_value in y_values:
                group_dict[y_value] = group_color
            color_idx += 1
    handles = []
    for y_value in sorted(color_dict.keys(), key=lambda x: len(color_dict[x]), reverse=True):
        handles.append(mpatches.Patch(color=group_dict[y_value], label=f'{y_value} ({len(color_dict[y_value])})'))
        for point in color_dict[y_value]:
            plt.scatter([point[0]], point[1], color=group_dict[y_value])
    plt.xlabel('Square size --->')
    plt.ylabel('Smallest rectangle (Ly value) --->')
    plt.title('Epsilon = ' + str(epsilon[j]))
    sm = ScalarMappable(cmap=cm.Blues, norm=plt.Normalize(vmin=0, vmax=len(count_dict)))
    sm.set_array([])
    #plt.colorbar(sm, orientation='vertical')
    plt.legend(title = "Frequency sort", handles=handles, loc = 'upper left', bbox_to_anchor=(1, 1))

    plt.show()


# %% [markdown]
# # Machine Learning

# %%
import pandas as pd
import numpy as np
import matplotlib.pyplot as plt
import seaborn as sns
from sklearn.model_selection import train_test_split
from sklearn.neighbors import KNeighborsRegressor
from sklearn.linear_model import Lasso
from sklearn.linear_model import ElasticNet
from sklearn.linear_model import LinearRegression
from sklearn.linear_model import RidgeCV

from sklearn.ensemble import ExtraTreesRegressor
from sklearn.ensemble import GradientBoostingRegressor
from sklearn.ensemble import RandomForestRegressor
from sklearn.ensemble import AdaBoostRegressor

from sklearn.tree import DecisionTreeRegressor
import lazypredict
from lazypredict.Supervised import LazyRegressor


from sklearn.multioutput import MultiOutputRegressor

# %% [markdown]
# # Prediction using shape values

# %%
# Prepare the data
final_data = []
square_size = [i for i in range(104,904,10)]
for i in square_size:
	ly_values = [b for b in range(2,i)]
	final_m_values = np.load("/home/rjoseph1/fftw++/tests/trial_runs/new_runs/final_square_m_values" + str(i) + ".npy").tolist()
	final_time_values = np.load("/home/rjoseph1/fftw++/tests/trial_runs/new_runs/final_square_time_values" + str(i) + ".npy").tolist()
	for m in range(len(ly_values)):
		for n in range(len(final_m_values[m])):	
			final_data.append([ly_values[m], ly_values[m]*2, i, 2*i, final_m_values[m][n], final_time_values[m][n]])


# %%
final_data = np.array(final_data)
dataset = pd.DataFrame({'Ly': final_data[:, 0], 'My': final_data[:, 1], 'Lx': final_data[:, 2], 'Mx': final_data[:, 3], 'm': final_data[:, 4], 'time': final_data[:, 5]})

# %%
dataset.info()

# %%
# ML part
X = dataset.drop(['m'], axis=1)
y = dataset[['m']]
X_train, X_test, y_train, y_test = train_test_split(X, y, test_size=0.0001, random_state=101)

reg = LazyRegressor(verbose=10, ignore_warnings=False, custom_metric=None)
models, predictions = reg.fit(X_train, X_test, y_train, y_test)

# %% [markdown]
# # Prediction using epsilon

# %%
def build(epsilon, non_optimal_square_size, array3, choice = 0):
	final = []
	for i in range(len(epsilon)):
		for j in range(len(array3[i])):
			final.append([epsilon[i], int(non_optimal_square_size[j]), 2*int(non_optimal_square_size[j])+choice, int(array3[i][j][0])])
	return np.array(final)

# %%
epsilon = [0.01, 0.0001, 0.001, 0.01, 0.05, 0.1, 0.12, 0.13, 0.2]
threshold = 2

# 1
non_optimal_square_size =  sorted(generate_multiples(a_max=10, b_max=10, c_max=10, d_max=10, bound = 1800))[2:] #list(filter(lambda x: x in multiples, values))
array3, array_final, array_x = square_optimal(non_optimal_square_size, threshold, epsilon, choice = 0)
final_data = build(epsilon, non_optimal_square_size, array3, choice = 0)
dataset = pd.DataFrame({'eps': final_data[:, 0], 'Lxy': final_data[:, 1], 'Mxy': final_data[:, 2], 'square': final_data[:, 3]})

# 2
#non_optimal_square_size =  sorted(generate_multiples(a_max=10, b_max=10, c_max=10, d_max=10, bound = 512))[2:] #list(filter(lambda x: x in multiples, values))
#array3, array_final, array_x = square_optimal(non_optimal_square_size, threshold, epsilon, choice = 1)
#final_data1 = build(epsilon, non_optimal_square_size, array3, choice = 1)
#dataset1 = pd.DataFrame({'eps': final_data[:, 0], 'Lxy': final_data1[:, 1], 'Mxy': final_data1[:, 2], 'square': final_data[:, 3]})

# 3
#non_optimal_square_size =  sorted(generate_multiples(a_max=10, b_max=10, c_max=10, d_max=10, bound = 512))[2:] #list(filter(lambda x: x in multiples, values))
#array3, array_final, array_x = square_optimal(non_optimal_square_size, threshold, epsilon, choice = 2)
#final_data2 = build(epsilon, non_optimal_square_size, array3, choice = -1)
#dataset2 = pd.DataFrame({'eps': final_data2[:, 0], 'Lxy': final_data2[:, 1], 'Mxy': final_data2[:, 2], 'square': final_data[:, 3]})


# 4 Combined
dataset_combined = pd.DataFrame({'eps': final_data[:, 0], 'Lxy': final_data[:, 1], 'Mxy': final_data[:, 2], 'square': final_data[:, 3]}) #'Mxy1': final_data1[:,2], 'square1': final_data1[:, 3], 'Mxy-1': final_data2[:,2], 'square2': final_data2[:, 3]})

# %%
# combine datasets
dataset_final = dataset #pd.concat([dataset, dataset1, dataset2], axis=0)

# %%
dataset.info

# %%
import matplotlib.pyplot as plt

plt.scatter(final_data2[:, 1], final_data[:, 3], label="Final Data")
plt.scatter(final_data2[:, 1], final_data1[:, 3], label="Final Data1")
plt.scatter(final_data2[:, 1], final_data2[:, 3], label="Final Data2")

plt.title("Scatter Plot of Final Data Sets")
plt.xlabel("Final Data2 Column 2 Values")
plt.ylabel("Final Data Column 3 Values")

plt.legend() # Add legend for data sets

plt.show()


# %% [markdown]
# # Manual Optimization

# %%
# ML part
X = dataset_final.drop(['square'], axis=1)
y = dataset_final[['square']]
X_train, X_test, y_train, y_test = train_test_split(X, y, test_size=0.0001, random_state=101)

# %%
from sklearn.model_selection import cross_val_score
from sklearn.ensemble import ExtraTreesClassifier, RandomForestClassifier, AdaBoostClassifier, GradientBoostingClassifier
from sklearn.neighbors import KNeighborsClassifier
from sklearn.linear_model import LogisticRegression, RidgeClassifier, Lasso, ElasticNet
from sklearn.tree import DecisionTreeClassifier
from sklearn.multioutput import MultiOutputClassifier

ESTIMATORS = {
    "Extra trees": ExtraTreesClassifier(n_estimators=100,
                                         max_features=5000,  # Out of 20000
                                         random_state=0),
    "K-nn": KNeighborsClassifier(),  # Accept default parameters
    "Logistic regression": LogisticRegression(),
    "Ridge": RidgeClassifier(),
    "Lasso": Lasso(),
    "ElasticNet": ElasticNet(random_state=0),
    "RandomForestClassifier": RandomForestClassifier(max_depth=100, random_state=2),
    "Decision Tree Classifier": DecisionTreeClassifier(max_depth=1000),
    "MultiO/P GBC": MultiOutputClassifier(GradientBoostingClassifier(n_estimators=100)),
    "MultiO/P AdaB": MultiOutputClassifier(AdaBoostClassifier(n_estimators=100))
}

best_score = -1e5
best_estimator = None

for name, estimator in ESTIMATORS.items():
    scores = cross_val_score(estimator, X_train, y_train, cv=5)
    mean_score = scores.mean()
    if mean_score > best_score:
        best_score = mean_score
        best_estimator = estimator

print("Best estimator: {}".format(best_estimator))
print("Best cross-validation score: {}".format(best_score))
best_estimator.fit(X_train, y_train)


# %%
from sklearn.model_selection import cross_val_score

ESTIMATORS = {
    "Extra trees": ExtraTreesRegressor(n_estimators=100,
                                       max_features=5000,     # Out of 20000
                                       random_state=0),
    "K-nn": KNeighborsRegressor(),                          # Accept default parameters
    "Linear regression": LinearRegression(),
    "Ridge": RidgeCV(),
    "Lasso": Lasso(),
    "ElasticNet": ElasticNet(random_state=0),
    "RandomForestRegressor": RandomForestRegressor(max_depth=100, random_state=2),
    "Decision Tree Regressor":DecisionTreeRegressor(max_depth=1000),
    "MultiO/P GBR" :MultiOutputRegressor(GradientBoostingRegressor(n_estimators=100)),
    "MultiO/P AdaB" :MultiOutputRegressor(AdaBoostRegressor(n_estimators=100))
}

best_score = -1e5
best_estimator = None

for name, estimator in ESTIMATORS.items():
    scores = cross_val_score(estimator, X_train, y_train, cv=10)
    mean_score = scores.mean()
    if mean_score > best_score:
        best_score = mean_score
        best_estimator = estimator

print("Best estimator: {}".format(best_estimator))
print("Best cross-validation score: {}".format(best_score))
best_estimator.fit(X_train, y_train)


# %%
X_test_final = X_test
y = best_estimator.predict(X_test)
score = best_estimator.score(X_test, y_test)
print("R^2 score: {:.4f}".format(score))

X_test_final['predict'] = y


# %%
X_test_final['actual'] = y_test['square'].astype(int)
X_test_final['diff'] = X_test_final['predict'] - X_test_final['actual']

# %%
pd.set_option('display.max_rows', 20)
X_test_final

# %% [markdown]
# # Now checking for OOD

# %%
epsilon = [0.0001, 0.001, 0.01, 0.05, 0.1, 0.12, 0.13, 0.2, 0.3, 0.4, 0.5, 0.6, 0.7, 0.8, 0.9]
non_optimal_square_size =  [i for i in range(128, 155)]
threshold = 2
array3, array_final, array_x = square_optimal(non_optimal_square_size, threshold, epsilon, choice = 0)

final = []
for i in range(len(epsilon)):
	for j in range(len(array3[i])):
		final.append([epsilon[i], int(non_optimal_square_size[j]), 2*int(non_optimal_square_size[j]), int(array3[i][j][0])])
final_data = np.array(final)
dataset = pd.DataFrame({'eps': final_data[:, 0], 'Lxy': final_data[:, 1], 'Mxy': final_data[:, 2], 'square': final_data[:, 3]})
X_test1, y_test1 = dataset.drop(['square'], axis=1), dataset[['square']]
y = best_estimator.predict(X_test1)
print("Score ", best_estimator.score(X_test1, y_test1))
X_test1['predict'] = y[:] #- y_test['square'].astype(int).to_numpy()
X_test1['actual'] = y_test1['square'].astype(int)
X_test1['diff'] = X_test1['predict'] - X_test1['actual']
X_test1

# %%
len(non_optimal_square_size)

# %% [markdown]
# # Check for 2,3,5,7

# %%
epsilon = [0.0001, 0.001, 0.01]
non_optimal_square_size1 =  sorted(generate_multiples(a_max=10, b_max=10, c_max=10, d_max=10, bound = 2048))[181:]
threshold = 2
array3, array_final, array_x = square_optimal(non_optimal_square_size1, threshold, epsilon, choice = 0)

final = []
for i in range(len(epsilon)):
	for j in range(len(array3[i])):
		final.append([epsilon[i], int(non_optimal_square_size[j]), 2*int(non_optimal_square_size[j]), int(array3[i][j][0])])
final_data = np.array(final)
dataset = pd.DataFrame({'eps': final_data[:, 0], 'Lxy': final_data[:, 1], 'Mxy': final_data[:, 2], 'square': final_data[:, 3]})
X_test1, y_test1 = dataset.drop(['square'], axis=1), dataset[['square']]
y = best_estimator.predict(X_test1)
print("Score ", best_estimator.score(X_test1, y_test1))
X_test1['predict'] = y[:] #- y_test['square'].astype(int).to_numpy()
X_test1['actual'] = y_test1['square'].astype(int)
X_test1['diff'] = X_test1['predict'] - X_test1['actual']
X_test1

# %%
X_test1

# %%

\end{lstlisting}
