# Supplementary material for: Hybrid Dealiased Convolutions
Source: arXiv:2306.10016 source file (2023-05-14)
Supplement: Supplementary file 2 [file appendix2.tex]

\section{Appendix}

\subsection{Main Algorithm}

\begin{algorithm}[H]
    \SetAlgoLined
    \DontPrintSemicolon
    \KwIn{F, f, m, L, p, q, r}
    \KwOut{Output signal $F$}
    $Q \gets \text{ceilquotient}(M, \lambda_1m)$\;
    
    \For{$\lambda_2 \gets 0$ \KwTo $\lambda_1 - 1$}{
        $W \gets$ array of size $m$ with complex zeros\;
        $R \gets Q\lambda_2 + r$\;
        
        \For{$s \gets 0$ \KwTo $m-1$}{
            $\text{sum} \gets 0$\;
            
            \For{$t \gets 0$ \KwTo $p-2$}{
                $\text{sum} \gets \text{sum} + f[tm + s]\exp\left(\frac{2\pi iR(tm + s)}{qm}\right)$\;
            }
            
            $W[s] \gets \text{sum}$\;
        }
        
        \For{$s \gets 0$ \KwTo $L - (p-1)m - 1$}{
            $W[s] \gets W[s] + f[(p-1)m + s]\exp\left(\frac{2\pi iR((p-1)m + s)}{qm}\right)$\;
        }
        
        $W \gets m*\mathcal{F}(W)$ \Comment*[r]{Compute the FFT of $W$ using $\mathcal{F}$}
        
        \For{$l \gets 0$ \KwTo $m-1$}{
            $F[\lambda_1l + \lambda_2] \gets W[l]$\;
        }
    }
    
    \Return{F}\;
    
    \caption{Forward Routine for 1D}\label{algo_forward}
\end{algorithm}

\begin{algorithm}[H]
\SetAlgoLined
\DontPrintSemicolon
\KwIn{F, f, m, L, p, q, r}
\KwOut{f}
$W \gets \mathcal{F}(F)$;

\For{$s \gets 0$ \KwTo $m-1$}{
    \For{$t \gets 0$ \KwTo $q-2$}{
        $f[tm + s] \gets f[tm + s] + W[s] * \overline{\exp\left(\frac{2\pi iR(tm + s)}{qm}\right)}$;
    }
}

\For{$s \gets 0$ \KwTo $L - (q-1)m - 1$}{
    $f[(q-1)m + s] \gets f[(q-1)m + s] + W[s] * \overline{\exp\left(\frac{2\pi iR((q-1)m + s)}{qm}\right)}$;
}
\Return{f};
\caption{Backward Routine for 1D}\label{algo_backward}
\end{algorithm}

\begin{algorithm}[H]
\DontPrintSemicolon
\SetKwInOut{Input}{Input}
\SetKwInOut{Output}{Output}
\Input{$f$, $g$, $m$, $L1$, $L2$, $\lambda$, $M1$}
\Output{$h_tilda$}
\caption{Main Convolution for 1D}
\vspace{0.2cm}

\tcp{declare variables and arrays}
$M_f \gets m$;

$M_g \gets M_f \cdot \lambda$;

$P_f \gets \left\lceil\frac{L_1}{M_f}\right\rceil$;

$P_g \gets \left\lceil\frac{L_2}{M_g}\right\rceil$;

$Q_g \gets \left\lceil\frac{M_1}{M_g}\right\rceil$;

$Q_f \gets \lambda \cdot Q_g$;

$Q_m \gets Q_f \cdot M_f$;

$M_1 \gets Q_g \cdot M_g$;

$m \gets M_g$;

$f \gets \text{concat}(f,\text{zeros}(P_f \cdot M_f - L_1))$;

$g \gets \text{concat}(g,\text{zeros}(P_g \cdot M_g - L_2))$;

$h_{tilda} \gets \text{zeros}(M_1)$;

$F \gets \text{zeros}(M_g)$;

$G \gets \text{zeros}(M_g)$;

$f_{final} \gets \text{zeros}(M1)$;

$g_{final} \gets \text{zeros}(M1)$;

$value \gets 0$;

\For{$r \gets 0$ \KwTo $Q_g-1$}{

$f_{final}[value:value+m] \gets \text{forward}(f,F,M_f,L_1,P_f,Q_f,r,\lambda,M_1)$;

$g_{final}[value:value+m] \gets \text{forward}(g,G,M_g,L_2,P_g,Q_g,r,\lambda,M_1)$;

$value \gets value + m$;
}

$f_{final} \gets f_{final} \cdot g_{final}$;

$f_{final} \gets f_{final}/Q_m$;

$value \gets 0$;

\For{$r \gets 0$ \KwTo $Q_g-1$}{

$h_{tilda} \gets \text{backward}(f_{final}[value:value+m],h_{tilda},M_g,M_1,P_g,Q_g,r)$;

$value \gets value + m$;
}

\label{mainconvolve}
\end{algorithm}

\subsection{Optimization Algorithms}

\begin{algorithm}[H]
\label{cross}
\SetAlgoLined
\KwIn{ESTIMATORS, X_{train}, y_{train}}
\KwOut{Best estimator and best cross-validation score}
best_{score} $\gets -\infty$;

best_{estimator} $\gets$ None;

\For{name, estimator \textbf{in} ESTIMATORS}{

scores $\gets$ cross_{validation-score}(estimator, X_{train}, y_{train}, cv=5);

mean_{score} $\gets$ scores.mean();

\If{mean_{score} > best_{score}}
{

best_{score} $\gets$ mean_{score};

best_{estimator} $\gets$ estimator;
}

}

\Return best_{estimator}.fit(X_{train}, y_{train});

\caption{Finding the best estimator using cross-validation}
\end{algorithm}

\begin{algorithm}[H]
\label{threshold}
\SetAlgoLined
\caption{Sort lists by threshold}
\KwIn{Lists $A$ and $B$, threshold parameter $\epsilon$}
\KwOut{Sorted lists $\text{sorted}A$ and $\text{sorted}B$}
Create a list of tuples $(a_i, b_i, i)$, where $a_i \in A$ and $b_i \in B$ and $i$ is the index of $b_i$ in $B$;

Sort the list of tuples based on the values in $B$;

Set $t_{\text{best}}$ to the value of $b_0$, the smallest value of $B$;

Set $t_{\text{worst}}$ to the value of $b_{n-1}$, the largest value of $B$;

Set the threshold $T$ to $t_{\text{best}} + \epsilon \cdot (t_{\text{worst}} - t_{\text{best}})$;

Create an empty list $\text{sorted}_A$;

Create an empty list $\text{sorted}_B$;

\ForEach{tuple $(a_i, b_i, i)$}{

\If{$b_i \leq T$}{
Append $a_i$ to $\text{sorted}A$;

Append $(b_i - t_{\text{best}})/(t_{\text{worst}} - t_{\text{best}})$ to $\text{sorted}_B$;

}
}
\Return $\text{sorted}_A$, $\text{sorted}_B$;
\end{algorithm}

\subsection{Data Generation And Plotting}

\begin{algorithm}[H]
\SetAlgoLined
\KwIn{$a_{max}$, $b_{max}$, $c_{max}$, $d_{max}$, $bound$}
\KwOut{A list of multiples of the form $2^a \cdot 3^b \cdot 5^c \cdot 7^d$ that are less than or equal to $bound$}
$multiples \gets \emptyset$;
\For{$a \gets 0$ \KwTo $a_{max}$}{
\For{$b \gets 0$ \KwTo $b_{max}$}{
\For{$c \gets 0$ \KwTo $c_{max}$}{
\For{$d \gets 0$ \KwTo $d_{max}$}{
$multiple \gets 2^a \cdot 3^b \cdot 5^c \cdot 7^d$;

\If{$multiple \leq bound$}{

$multiples \gets multiples \cup {multiple}$;
}
}
}
}
}
\Return{$\text{list}(multiples)$};
\caption{Generate all the multiples}
\end{algorithm}

\begin{algorithm}[H]
\SetKwInOut{Input}{Input}
\SetKwInOut{Output}{Output}

\Input{A regex pattern $pattern$ and a string $line$}

\Output{A list $m$ of floats}

$m \leftarrow$ empty list\;

$matches \leftarrow$ find all non-overlapping matches of $pattern$ in $line$\;

\For{each $match$ in $matches$}{
	$number \leftarrow$ the substring of $match$ starting from the third character\;
 
	$float\_number \leftarrow$ convert $number$ to a float\;
 
	append $float\_number$ to $m$\;
}
\Return{$m$}\;

\caption{Match Pattern for Data generation}
\end{algorithm}
